# Supplementary material for: Proximal Causal Inference for Complex Longitudinal Studies
Source: arXiv:2109.07030 source file (2022-08-03)
Supplement: Supplementary file 1 [file suppmnotation.tex]

% specific

% specific

%\def\I{\mathscr{I}}

% environments

\numberwithin{thm}{section}

\numberwithin{prp}{section}

\numberwithin{lem}{section}

\numberwithin{cor}{section}

\numberwithin{assump}{section}

\theoremstyle{remark}

\numberwithin{Def}{section}

\numberwithin{rem}{section}

\def\beq{\begin{equation}} % \setcounter{equation}{1}}
\def\eeq{\end{equation}}
\def\beqn{\begin{eqnarray*}}
\def\eeqn{\end{eqnarray*}}
\def\Bitem{\begin{itemize}\setlength{\itemsep}{.2in}}
\def\bitem{\begin{itemize}\setlength{\itemsep}{.05in}}
\def\eitem{\end{itemize}}
\def\Benum{\begin{enumerate}\setlength{\itemsep}{.2in}}
\def\benum{\begin{enumerate}\setlength{\itemsep}{.05in}}
\def\eenum{\end{enumerate}}
\def\bmult{\begin{multline*}}
\def\emult{\end{multline*}}
\def\bcenter{\begin{center}}
\def\ecenter{\end{center}}
\def\bframe{\begin{frame}}
\def\eframe{\end{frame}}

% references

% operators

%\DeclareMathOperator{\det}{det}

%\DeclareMathOperator{\span}{span}

% functions

% cal letters

% bold letters (upper case)

% bold letters (lower case)

% bold greek letters

% bb letters

% probability

%\newcommand{\cor}[1]{\operatorname{Cor}\left(#1\right)}

% other symbols

%\def\vol{{\rm vol}}

\def\1{\mathbbm{1}}
